# Supplementary material for: Higher-order topological insulators in amorphous solids
Source: arXiv:1902.00507 source file (2020-03-18)
Supplement: Supplementary file 1 [file HOTI_SM.pdf]

# Supplemental Material: Higher Order Topological Insulators in Amorphous Solids

Adhip Agarwala,[1,2] Vladimir Juričić,[3] and Bitan Roy[2,4]

[1]International Centre for Theoretical Sciences, Tata Institute of Fundamental Research, Bengaluru 560089, India
[2]Max-Planck-Institut für Physik komplexer Systeme, Nöthnitzer Str. 38, 01187 Dresden, Germany
[3]Nordita, KTH Royal Institute of Technology and Stockholm University, Roslagstullsbacken 23, 10691 Stockholm, Sweden
[4]Department of Physics, Lehigh University, Bethlehem, Pennsylvania, 18015, USA

## I. HOTI IN A COMPLETELY AMORPHOUS NETWORK

In a crystalline setup the term proportional to $g$, see Eq. (1) of the main text, breaks the $C_4$ symmetry and induces a HOTI phase. We generalize this coupling in an amorphous setting to $\sim g\,[\cos(2\phi) + i\alpha \sin(2\phi)]$. In the main part of the paper, we set $\alpha = 1$. Here we show the role of the parameter $\alpha$ in realizing a HOTI phase in a completely amorphous setup. Note that for any arbitrary value of $\alpha$ the above term breaks $C_4$ symmetry, as $g\,[\cos(2\phi) + i\alpha \sin(2\phi)] \rightarrow -g\,[\cos(2\phi) + i\alpha \sin(2\phi)]$ when $\phi \rightarrow \phi + \pi/2$. For the sake of concreteness we choose $0 \leq \alpha \leq 1$. Results are displayed in Figs. 1 and 2.

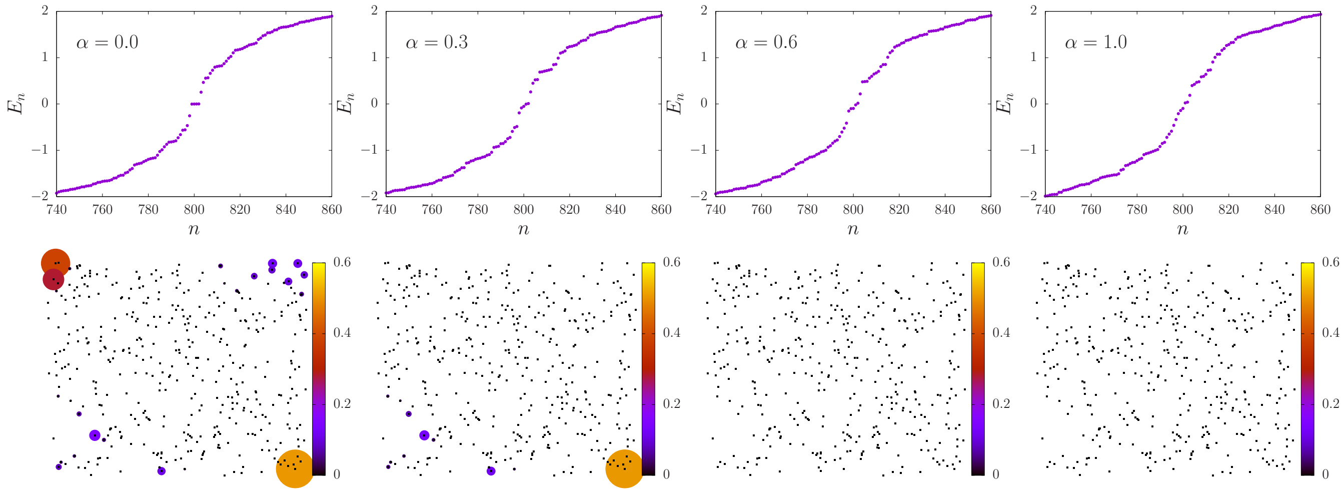


FIG. 1: Energy spectra (top row) and the local density of states (LDoS) corresponding to the corner modes (bottom row) (from left to right) in a system with a linear dimension $L = 20$ for $\alpha = 0.0, 0.3, 0.6$ and $1.0$. We set $R = 4, M = 0, g = 1, r_o = 1$ (see main text for definition of these parameters). In the top row $n$ is the index for energy eigenvalues $E_n$. The LDoS is calculated by the spectral weight within the window of 0.025 around the Fermi energy ($-0.025 < E - E_F < 0.025$) in a half-filled system. For the last two panels there are no states in the energy window to contribute to the spectral weight. The corresponding scaling of the quadrupolar moment ($Q_{xy}$) is shown in Fig. 2.

We note that *only* when $\alpha = 0$, even a completely amorphous network accommodates four degenerate states at zero energy with open boundary conditions in all directions. They contribute to a local density of states (LDoS) with spectral weight highly localized on four corners of the lattice (see Fig. 1), and we find that the quadrupolar moment $Q_{xy} = 0.5$ (within numerical accuracy) with both open and periodic boundaries (see Fig. 2). We then realize a HOTI in a completely amorphous system. Tuning a finite value of $\alpha$ mixes these corner states and the quasidengeneracy of the corner modes is lost. This in turn removes the fact that the LDoS is sharply localized at the four corners and $Q_{xy}$ is no longer pinned at its quantized value 0.5. The system is then not an amorphous HOTI. The singular behavior at $\alpha = 0$ can be justified in the following way. Note that in our construction even the fully amorphous system retains an overall square shape, and when $\alpha = 0$ the $C_4$ symmetry breaking perturbation vanishes along the diagonals of the system that also include four corners. Consequently, even though there exists no sites precisely at a corner, the spectral weight of the corner mode gets localized in its close vicinity, see for example Fig. 1 (leftmost column), and concomitantly we find $Q_{xy} = 0.5$ with both periodic and open boundaries, see Fig. 2. Therefore we realize a completely amorphous HOTI. Any finite $\alpha$ causes mixing of such corner states with the bulk state and even for a small value of $\alpha$ corner states melt and we loose amorphous HOTI. To compare these findings, next we test the stability of crystalline (free of any structural disorder) HOTI with varying $\alpha$, see Fig. 3.

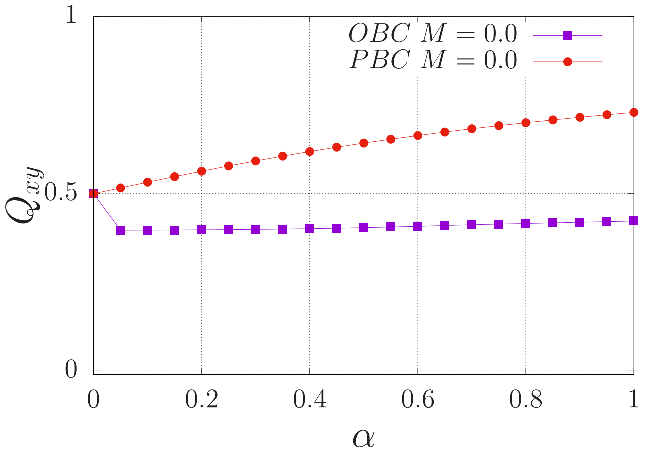


FIG. 2: Variation of the quadrupolar moment $Q_{xy}$ (defined modulo 1) as a function of $\alpha$ (see text) with both open boundary condition (OBC) and periodic boundary condition (PBC). Rest of the parameters are same as in Fig. 1. Note that only for $\alpha = 0$ we have $Q_{xy} = 0.5$ (within numerical accuracy) for both PBC and OBC, and we realize a completely amorphous HOTI.

## II. CRYSTALLINE HOTI

In a perfectly crystalline setup with only nearest neighbor bonds variation of $\alpha$ makes no difference to either the spectra (see Fig. 3) or the value of $Q_{xy}$ (see Fig. 4). To illustrate this explicitly we show the energy spectra and the LDoS, corresponding to the corner modes in Fig. 3 for various choices of $\alpha$. Furthermore, in Fig. 4 we show the variation of $Q_{xy}$ with $\alpha$ for four different values of $M$. Note that $Q_{xy}$ remains quantized to 0.5(0.0) (within numerical accuracy) when the system is in HOTI (trivial) phase for both periodic and open boundaries in the system.

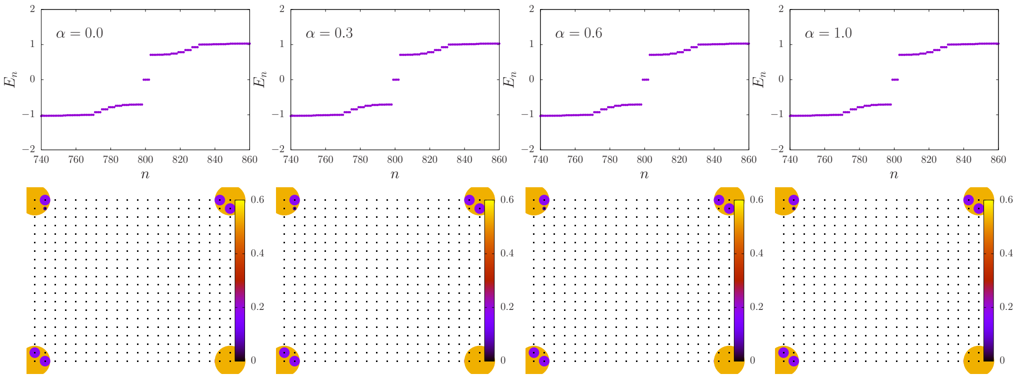


FIG. 3: Energy spectra (top row) and the local density of states (LDoS) for zero energy corner modes (bottom row) (from left to right) in a crystalline system with a linear dimension $L = 20$ and for $\alpha = 0.0, 0.3, 0.6$ and 1.0. For numerical computation we set $R = 1, M = -1.0, g = 1, r_o = 1$. In the top row $n$ is the index for energy eigenvalues $E_n$. The LDoS is calculated by the spectral weight within the window of 0.025 around the Fermi energy ($-0.025 < E - E_F < 0.025$) in a half-filled system.

## III. ROBUSTNESS OF QUADRUPOLAR MOMENT $Q_{xy}$

In order to investigate the role of the boundary conditions in the computation of the quadrupolar moment ($Q_{xy}$), we consider the following (specifically 8) cases, for which the system is expected to be in the HOTI regime (as it supports four near zero-energy corner modes with open boundaries). These amount to

1. changing the extension of the lattice ($L$) to even and odd number of sites,

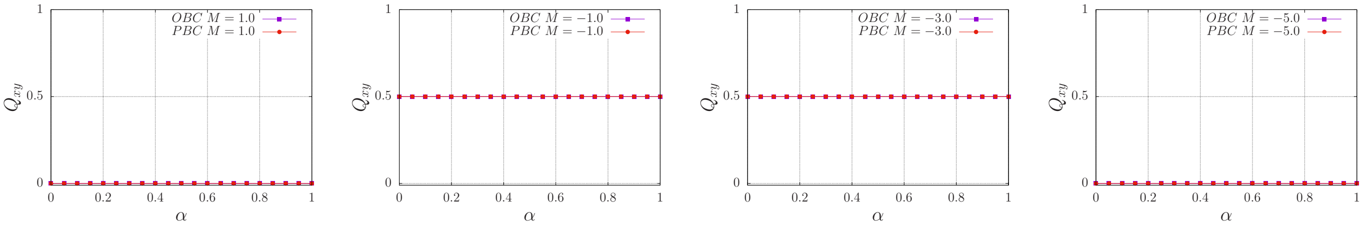


(a) (b) (c) (d)

FIG. 4: Variation of the quadrupolar moment $Q_{xy}$ as a function of $\alpha$ for four specific values of $M$, namely (a) $M = 1.0$, (b) $M = -1.0$, (c) $M = -3.0$ and (d) $M = -5.0$. For numerical analysis we set $R = 1, g = 1, r_o = 1$.

| Type | $L = 20$ | $Q_{xy}$ (PBC) | $Q_{xy}$ (OBC) | $L = 21$ | $Q_{xy}$ (PBC) | $Q_{xy}$ (OBC) |
|---|---|---|---|---|---|---|
| I | 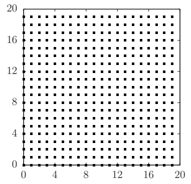 | 0.499997871 | 0.499997868 | 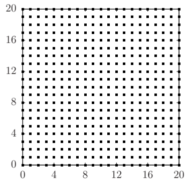 | 0.499997593 | 0.499997623 |
| II | 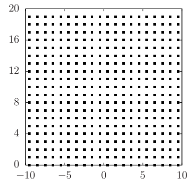 | 0.499999986 | 0.499999976 | 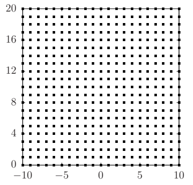 | 0.500000014 | 0.500000066 |
| III | 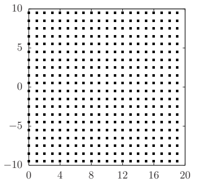 | 0.500000014 | 0.499999976 | 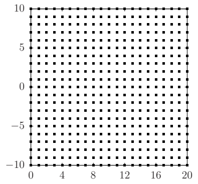 | 0.499999986 | 0.500000065 |
| IV | 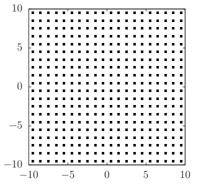 | **0.0** | **0.0** | 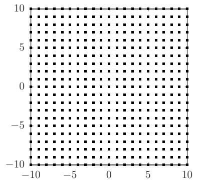 | **0.0** | **0.0** |

TABLE I: Quadrupolar moment ($Q_{xy}$) in a crystalline HOTI phase (obtained for $M = -1$ and $g = 1$). Respectively for I, II and III, the origin is chosen to be at the corner, at the center of the $x$ and $y$ axes, while for IV it is located at the center of the system. We compute $Q_{xy}$ in a system of even ($L = 20$) and odd ($L = 21$) dimensions, and with periodic boundary condition (PBC) and open boundary condition (OBC).

2. shifting the position of real space origin to various (specifically 4) positions of the lattice (for each choice of $L$).

For each such choice we compute $Q_{xy}$ using the protocol, chalked out in the main text of the manuscript. We perform this analysis for both crystalline and amorphous (with $L \gg R$) systems, for which the results are summarized in Table I and Table II, respectively. For the crystalline system, we always set $M = -1, g = 1$, whereas for the amorphous one we take $M = 0, g = 1, R = 4, R_s = 6, r_0 = 1$. For these choices of the parameters, the (crystalline or amorphous) system of linear dimension $L = 20$ or 21 in the $x$ and $y$ direction supports four near zero-energy corner modes (in open systems), and thus expected to be in the HOTI phase with quantized $Q_{xy} = 0.5$ (within numerical accuracy).

First of all, the cases analyzed in Table I and Table II, it appears that $Q_{xy}$ does not depend

1. on the choice of boundary condition (periodic or open),

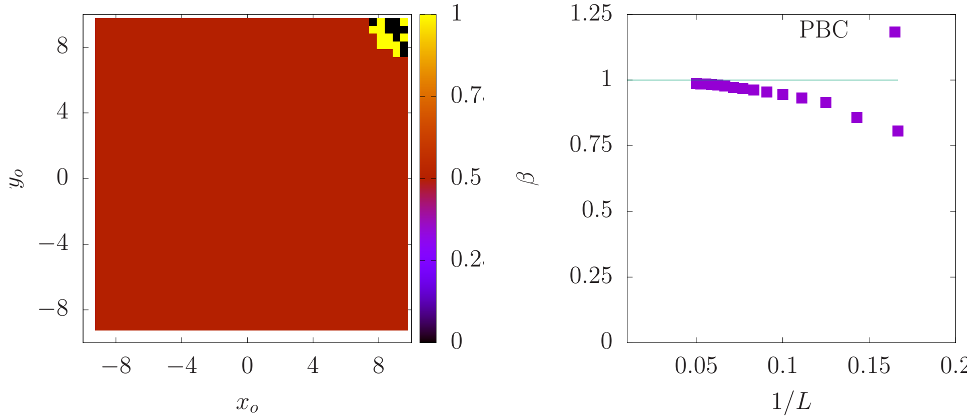


FIG. 5: (Left) Contour plot of $Q_{xy}$ (for $M = -1, g = 1$) for a crystalline HOTI in the range of $x_o$ and $y_o$ (with periodic boundaries). The positions of the lattice sites are given by $\{x_i - x_o, y_i - y_o\}$ and $0 \leq \{x_i, y_i\} \leq L = 20$. Here, $x_o$ and $y_o$ are chosen in intervals of $0.5a$. (Right) The fraction of area where $Q_{xy}$ is $0.5 \pm 10^{-3}$ is given by $\beta$, and the variation of $\beta$ as a function of $1/L$ shows that it saturates to 1 in the thermodynamic limit ($L \to \infty$). Hence, in the thermodynamic limit $Q_{xy}$ in the crystalline HOTI phase is independent of the choice of origin.

2. on the choice of linear dimension of the system ($L$) being even or odd.

We also note that for most of the choices of the origin, such as when it is located at the corner of the system, and at the center of the $x$ and $y$ axes, $Q_{xy}$ is quantized to at least $0.5 \pm 10^{-5}$ (for the crystalline system) and $0.5 \pm 10^{-2}$ (for the amorphous system), see I, II and III of Table I and Table II. However, when the origin is chosen to be at (or around) the center of the system $Q_{xy} \neq 0.5$, even though the spectra do not depend on the choice of origin. Therefore, from these analyses we observe that for reasonably large system sizes $Q_{xy}$ does not appear to depend on the choice of boundary condition and whether $L$ is even or odd for both crystalline and amorphous systems.

For the quadrupolar moment ($Q_{xy}$) to qualify as a bonafide topological order parameter to characterize HOTIs (crystalline and amorphous), it must be independent of the choice of the origin. In this context, we note that any topological order parameter, such as the first Chern number or the Bott index, is strictly defined in a system with periodic boundary. Hence, from now on we only focus on periodic systems, and show that in the thermodynamic limit (as $L \to \infty$) $Q_{xy}$ does not depend on the choice of the origin in crystalline and amorphous systems.

In order to completely characterize its origin dependency, we start from the configuration of Type I (for both crystalline and amorphous systems) and evaluate $Q_{xy}$ by displacing all positions by a shift of origin $\{x_o, y_o\}$. We fine grid the choice of $\{x_o, y_o\}$ in units of $0.5a$ where $a$ is the microscopic length scale characterizing the lattice spacing and evaluate $Q_{xy}$ in this phase region of $\{x_o, y_o\}$ as shown in Fig. 5. We introduce a quantity $\beta$, measuring the fraction of the area in the $\{x_o, y_o\}$ plane, where $Q_{xy}$ is 0.5 (within numerical accuracy), and examine the scaling of $\beta$ with $1/L$.

For crystalline system the results are displayed in Fig. 5. We find that $\beta \to 1$, as we approach the thermodynamic limit ($L \to \infty$). We now turn our focus to the amorphous system, where the interior region is scrambled. Given a system of dimension $L \times L$, the diameter of the disordered region with is chosen to be $R_s = (L/2) - 4$, such that fraction of the system that gets scrambled remains (almost) constant. We find that $\beta \to 1$ as $L \to \infty$, as shown in Fig. 6. Note that in this analysis $L$ is chosen to be both even and odd. Therefore, in the true thermodynamic limit $Q_{xy} = 0.5$ (within numerical accuracy) becomes independent of the choice of the origin in a system with periodic boundary and therefore it qualifies as a bonafide topological order parameter to identify a two-dimensional HOTI, in both crystalline and amorphous systems.

Next we turn our focus to the crystalline and amorphous trivial insulators, for which $Q_{xy} = 0$. For numerical analyses we choose $M = 8$ for both crystalline and amorphous systems, leaving the other parameter values unchanged. We always find that in periodic system $Q_{xy} = 0$ for all choices of the origin and for any system size $L$. Hence, for trivial insulator $\beta = 1$ for any $L$. Therefore, the quadrupolar moment besides being independent of the choice of origin, also distinguishes HOTI and trivial insulator in both crystalline and amorphous systems. Due to such featureless dependence of $Q_{xy} = 0$ in the trivial insulating phase with boundary condition and system size, we do not show the results explicitly. In a similar fashion, we expect that the octupolar moment $Q_{xyz} = 0.5$ and 0 in a three-dimensional HOTI (crystalline and amorphous) and trivial insulating phases, respectively, do not depend on the choice of origin in the thermodynamic limit.

| Type | $L = 20$ | $Q_{xy}$ (PBC) | $Q_{xy}$ (OBC) | $L = 21$ | $Q_{xy}$ (PBC) | $Q_{xy}$ (OBC) |
|---|---|---|---|---|---|---|
| I | 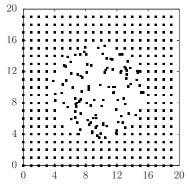 | 0.495233707 | 0.494257414 | 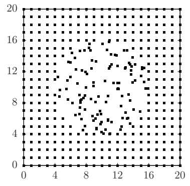 | 0.489799042 | 0.489878998 |
| II | 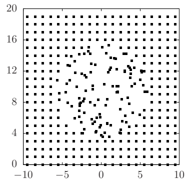 | 0.502232576 | 0.497310525 | 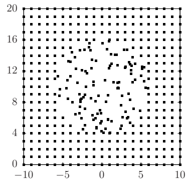 | 0.498181348 | 0.494242177 |
| III | 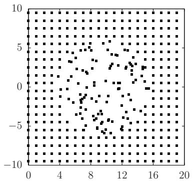 | 0.49766836 | 0.489557791 | 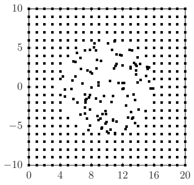 | 0.494992973 | 0.488981561 |
| IV | 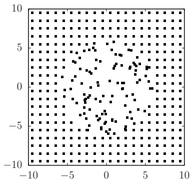 | **0.999451063** | **0.022545391** | 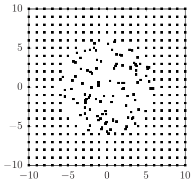 | **0.998652945** | **0.024656386** |

TABLE II: Same as Table I, but in an amorphous HOTI phase (obtained for $M = 0, g = 1, R = 4, R_s = 6, r_0 = 1$).

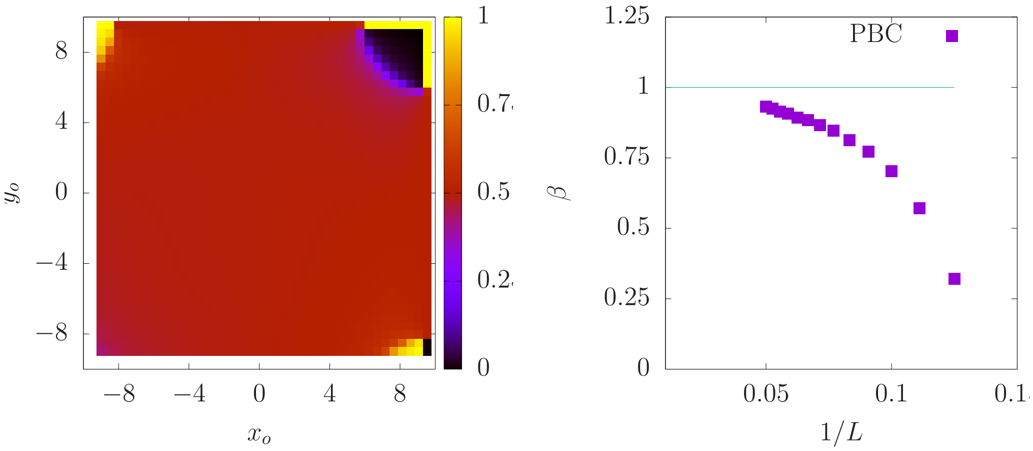


FIG. 6: (Left) Contour plot of $Q_{xy}$ for an amorphous HOTI (for $M = 0, g = 1, R = 4, r_0 = 1$) in the range of $x_o$ and $y_o$ (with periodic boundaries). The positions of the lattice sites are given by $\{x_i - x_o, y_i - y_o\}$ and $0 \leq \{x_i, y_i\} \leq L = 20$. For every $L$, we choose the scrambling radius to be $R_s = (L/2) - 4$, such that fraction of the system that is scrambled remains (almost) constant. Here, $x_o$ and $y_o$ are chosen in intervals of $0.5a$. (Right) The fraction of area of this region where $Q_{xy}$ is within $0.5 \pm 0.05$ is given by $\beta$. Variation of $\beta$ as a function of $1/L$ shows that it saturates to 1 in the thermodynamic limit ($L \to \infty$). Hence, in an amorphous HOTI phase, $Q_{xy}$ is independent of the choice of origin in the thermodnamic limit.
